# Supplementary material for: Fine-Grained Socioeconomic Prediction from Satellite Images with Distributional Adjustment
Source: arXiv:2308.15979 source file (2023-09-04)
Supplement: Supplementary file 1 [file appendix.tex]

\appendix
